# Supplementary material for: Adaptive Optimization Algorithms for Machine Learning
Source: arXiv:2311.10203 source file (2023-11-16)
Supplement: Supplementary file 1 [file Appendix_B.tex]

% Appendix B File

\refstepcounter{chapter}%
\chapter*{\thechapter \quad SGN Appendix} \label{ap:}

\subsection{Basic facts}
For any vectors $a, b\in\R^d$ and scalar $\nu>0$, Young's inequality states that
\begin{align}
    2\<a, b>\le \nu\|a\|^2+ \frac{1}{\nu}\|b\|^2. \label{eq:young}
\end{align}
Moreover, we have
\begin{align}
    \|a+b\|^2
    \le 2\|a\|^2 + 2\|b\|^2.\label{eq:a_plus_b}
\end{align}
More generally, for a set of $m$ vectors $a_1,\dotsc, a_m$ with arbitrary $m$, it holds
\begin{align}
    \Bigl\|\frac{1}{m}\sum_{i=1}^m a_i\Bigr\|^2
    \le \frac{1}{m}\sum_{i=1}^m\|a_i\|^2. \label{eq:jensen_for_sq_norms}
\end{align}
For any random vector $X$ we have
\begin{align}
    \ec{\|X\|^2}=\|\ec{X}\|^2 + \ec{\|X-\ec{X}\|^2}. \label{eq:rand_vec_sq_norm}
\end{align}
If $f$ is $L_f$--smooth, then for any $x,y\in\R^d$, it is satisfied
\begin{equation}
	f(y)
	\le f(x) + \<\nabla f(x), y-x> + \frac{L_f}{2}\|y-x\|^2. \label{eq:smooth_func_vals}
\end{equation}

Finally, for $L_f$--smooth and convex function $f$, it holds
\begin{equation}
f(x) \leq f(y)+\langle\nabla f(x), x-y\rangle-\frac{1}{2 L_f}\|\nabla f(x)-\nabla f(y)\|^{2} \label{eq:smooth_conv}.
\end{equation}

\begin{proposition} \label{pr:three_point} [Three-point identity]
	For any $u,v,w \in \R^d$, any $f$ with its Bregman divergence $D_f(x,y) = f(x)-f(y) - \langle \nabla f(y), x-y\rangle $, it holds
	\begin{align*}
	\langle \nabla f(u) - \nabla f(v), w-v \rangle
	&= D_f (v,u) + D_f(w,v) - D_f(w,u).
	\end{align*}
\end{proposition}

\begin{lemma}[Arithmetic mean -- Geometric mean inequality]
		For $c\geq0$ we have 
		\begin{equation} %\label{eq:AG}
		1+ c = \frac {1 + (1+2c)}{2} \stackrel{AG} \geq \sqrt{1+2c}.
		\end{equation}
	\end{lemma}
	
	\begin{lemma}[Jensen for square root]
		Function $f(x) = \sqrt x$ is concave, hence for $c\geq0$ we have 
		\begin{equation}\label{eq:jensen}
		\frac 1 {\sqrt 2} (\sqrt c+1) \leq \sqrt{c+1} \qquad \leq \sqrt c + 1.
		\end{equation}
	\end{lemma}
